# Supplementary material for: Huge Spin-Driven Polarizations at Room-Temperature in bulk BiFeO3
Source: arXiv:1504.07106 source file (2015-04-27)
Supplement: Supplementary file 1 [file striction_supp_prl.pdf]

# Supplemental Materials for "Huge Spin-Driven Polarizations at Room-Temperature in bulk $BiFeO_3$"

Jun Hee Lee and Randy S. Fishman
*Materials Science and Technology Division, Oak Ridge National Laboratory, Oak Ridge, Tennessee 37831, USA*
(Dated: April 24, 2015)

PACS numbers: 75.25.-j, 75.30.Ds, 75.50.Ee, 78.30.-j

## I. Theoretical Methods

### a. Microscopic spin model

While the FE ($\Gamma_4^-[111]$) distortion breaks inversion symmetry globally, the AFD ($R_4^+[111]$) distortion does so only locally in $R3c$ $BiFeO_3$. Each distortion creates its own Dzyaloshinskii-Moriya (DM) interaction, $\boldsymbol{D}_{\rm FE}$ and $\boldsymbol{D}_{\rm AFD}$. An updated microscopic spin model reflects the separate effect of each distortion:

$$\mathcal{H} = \mathcal{H}^{\rm EX} + \mathcal{H}^{\rm DM} + \mathcal{H}^{\rm SIA} \tag{1}$$

$$\mathcal{H}^{\rm EX} = -J_1 \sum_{\langle i,j\rangle} \mathbf{S}_i \cdot \mathbf{S}_j \tag{2}$$

$$\mathcal{H}^{\rm DM} = \mathcal{H}^{\rm DM}_{\rm FE} + \mathcal{H}^{\rm DM}_{\rm AFD} = \sum_{\mathbf{R}_i,\mathbf{R}_j=\mathbf{R}_i+\mathbf{e}_k} \boldsymbol{D}_{{\rm FE},k} \cdot (\mathbf{S}_i \times \mathbf{S}_j) + \sum_{\mathbf{R}_i,\mathbf{R}_j=\mathbf{R}_i+\mathbf{e}_k} (-1)^{n_i} \boldsymbol{D}_{{\rm AFD},k} \cdot (\mathbf{S}_i \times \mathbf{S}_j) \tag{3}$$

$$\mathcal{H}^{\rm SIA} = -K \sum_i (\mathbf{S}_i \cdot \mathbf{z}')^2, \tag{4}$$

where the $\boldsymbol{D}_{{\rm FE},k}$ and $\boldsymbol{D}_{{\rm AFD},k}$ terms involve vectors $\mathbf{e}_k = a\mathbf{x}$, $a\mathbf{y}$, and $a\mathbf{z}$ connecting neighboring sites $\mathbf{R}_i$ and $\mathbf{R}_j = \mathbf{R}_i + \mathbf{e}_k$ and the FE polarization is assumed to lie along $\mathbf{z}' = [1,1,1]$. Hexagonal layers normal to $\mathbf{z}'$ are separated by $c = a/\sqrt{3}$ and are labeled by the integers $n_i = \mathbf{R}_i \cdot \mathbf{z}'/c$. The coefficient $(-1)^{n_i}$ in front of $\boldsymbol{D}_{\rm AFD}$ reflects the alternating nature of the $R_4^+[111]$ AFD distortions from one hexagonal layer to the next. By contrast, the FE distortion and its DM interaction are translation-invariant.

Since the FE vectors $D^{\gamma}_{{\rm FE},k}$ are given by (0, $D_{\rm FE}$, $-D_{\rm FE}$) ($\gamma = x$), ($-D_{\rm FE}$, $D_{\rm FE}$, 0) ($\gamma = y$), and ($D_{\rm FE}$, $-D_{\rm FE}$, 0) ($\gamma = z$) between nearest spins along $x$,$y$, and $z$, resepctively in $R3c$ $BiFeO_3$ , we can transform the FE-induced DM interaction:

$$\mathcal{H}^{\rm DM}_{\rm FE} = \sum_{\mathbf{R}_i,\mathbf{R}_j=\mathbf{R}_i+\mathbf{e}_k} \boldsymbol{D}_{{\rm FE},k} \cdot (\mathbf{S}_i \times \mathbf{S}_j) = \sqrt{2}D \sum_{\mathbf{R}_i,\mathbf{R}_j=\mathbf{R}_i+\mathbf{e}_k} (\mathbf{z}' \times \mathbf{e}_k/a) \cdot (\mathbf{S}_i \times \mathbf{S}_j), \tag{5}$$

where $D_{\rm FE}$ = 89.0 nC/cm$^2$ from our LSDA+$U$ calculation. Although the $D$ term is now written as a sum over first-nearest neighbors, the $\sqrt{2}$ in front of $D$ guarantees that the DM energy is the same as given elsewhere [1] as a sum over second-nearest neighbors within each hexagonal plane. From Eq. 5, $D$=$\sqrt{(3/2)}D_{\rm FE}$=109 meV is very similar to previous determination (0.126 meV [7, 8]).

The AFD interactions $\boldsymbol{D}_{{\rm AFD},k}$ can be written

$$\boldsymbol{D}_{{\rm AFD},x} = B(\mathbf{y} + \mathbf{z}) + A\mathbf{x}, \tag{6}$$

$$\boldsymbol{D}_{{\rm AFD},y} = B(\mathbf{z} + \mathbf{x}) + A\mathbf{y}, \tag{7}$$

$$\boldsymbol{D}_{{\rm AFD},z} = B(\mathbf{x} + \mathbf{y}) + A\mathbf{z}. \tag{8}$$

$$\tag{9}$$

For the magnetic domain 2 [2] with wavevector along [1,0,-1],

$$\begin{aligned}
\mathcal{H}^{\rm DM}_{\rm AFD} &= \sum_{\mathbf{R}_i,\mathbf{R}_j=\mathbf{R}_i+\mathbf{e}_k} (-1)^{n_i} \boldsymbol{D}_{{\rm AFD},k}\cdot(\mathbf{S}_i\times\mathbf{S}_j) \qquad (10)\\
&= \sqrt{3}\sum_{\mathbf{R}_i}{}' \mathbf{z}'\cdot\Big\{B\,\mathbf{S}_r\times(\mathbf{S}_{\mathbf{R}_i+a\mathbf{x}}+2\mathbf{S}_{\mathbf{R}_i+a\mathbf{y}}+\mathbf{S}_{\mathbf{R}_i+a\mathbf{z}})+A\,\mathbf{S}_{\mathbf{R}_i}\times(\mathbf{S}_{\mathbf{R}_i+a\mathbf{x}}+\mathbf{S}_{\mathbf{R}_i+a\mathbf{z}})\Big\}\\
&+ \sum_{\mathbf{R}_i}{}' \mathbf{y}\cdot\Big\{(B-A)\mathbf{S}_{\mathbf{R}_i}\times(\mathbf{S}_{\mathbf{R}_i+a\mathbf{x}}-2\mathbf{S}_{\mathbf{R}_i+a\mathbf{y}}+\mathbf{S}_{\mathbf{R}_i+a\mathbf{z}})\Big\} \qquad (11)\\
&\approx \sqrt{3}\sum_{\mathbf{R}_i}{}' \mathbf{z}'\cdot\Big\{B\,\mathbf{S}_{\mathbf{R}_i}\times(\mathbf{S}_{\mathbf{R}_i+a\mathbf{x}}+2\mathbf{S}_{\mathbf{R}_i+a\mathbf{y}}+\mathbf{S}_{\mathbf{R}_i+a\mathbf{z}})+A\,\mathbf{S}_{\mathbf{R}_i}\times(\mathbf{S}_{\mathbf{R}_i+a\mathbf{x}}+\mathbf{S}_{\mathbf{R}_i+a\mathbf{z}})\Big\}, \qquad (12)\\
&\approx \sqrt{3}(4B+2A)\sum_{\mathbf{R}_i}{}' \mathbf{z}'\cdot(\mathbf{S}_{\mathbf{R}_i}\times\mathbf{S}_{\mathbf{R}_i+a\mathbf{y}}) \qquad (13)
\end{aligned}$$

where the primed sum over $\mathbf{R}_i$ is restricted to either $n_i$ odd or even hexagonal layers. Because the $\mathbf{y}$ term is of order $\delta^2 \sim 2\times10^{-5}$, the $\mathbf{z}'$ term dominates.

Previously [2], the second DM term was written

$$\begin{aligned}
\mathcal{H}^{\rm DM}_{\rm AFD} &= D' \sum_{\mathbf{R}_i,\mathbf{R}_j=\mathbf{R}_i+\mathbf{e}_k} (-1)^{n_i}\mathbf{z}'\cdot(\mathbf{S}_i\times\mathbf{S}_j) \qquad (14)\\
&= 2\sqrt{3}D'\sum_{\mathbf{R}_i}{}' \mathbf{z}'\cdot(\mathbf{S}_{\mathbf{R}_i}\times\mathbf{S}_{\mathbf{R}_i+a\mathbf{x}}+\mathbf{S}_{\mathbf{R}_i}\times\mathbf{S}_{\mathbf{R}_i+a\mathbf{y}}+\mathbf{S}_{\mathbf{R}_i}\times\mathbf{S}_{\mathbf{R}_i+a\mathbf{z}}) \qquad (15)\\
&\approx 6\sqrt{3}D'\sum_{\mathbf{R}_i}{}' \mathbf{z}'\cdot(\mathbf{S}_{\mathbf{R}_i}\times\mathbf{S}_{\mathbf{R}_i+a\mathbf{y}}) \qquad (16)
\end{aligned}$$

Therefore, $D' = (A+2B)/3 = 0.064$ meV ($A$=0.042, $B$=0.075 from our LSDA+$U$ calculations), which shows an excellent agreement with previous determinations of $D'$ (0.054 meV) [7, 8].

## b. First-principles calculations

First-principles calculations were performed using density functional theory (DFT) from the VASP code within a local spin-density approximation with an additional Hubbard (LSDA+$U$) for the exchange-correlation functional. The Hubbard parameter $U$ and the exchange interaction $J_{\rm H}$ were set to $U = 5$ eV and $J_{\rm H} = 0$ eV for $Fe^{3+}$, parameters that were found to be optimal for $BiFeO_3$ [3, 4]. We used the projector augmented wave (PAW) potentials [5]. While the magnetic coupling parameters (exchange, DM, SIA) depend on the choice of $U$ and $J_{\rm H}$, their derivatives with respect to an electric field are much less dependent. To integrate over the Brillouin zone, we used a supercell made of a 2×2×2 perovskite units (40 atoms, 8 f.u.), 3×3×3 Monkhorst-Pack (MP) $k$-points mesh. To evaluate $\boldsymbol{D}_{\rm FE}$ we employed a 4×2×2 unit (80 atoms, 16 f.u.) with a 1×3×3 Monkhorst-Pack (MP) mesh. The wave functions were expanded with plane waves up to an energy cutoff of 500 eV. To calculate exchange interactions ($J_\perp$, $J_\parallel$), we used four different magnetic configurations ($G$-,$C$-,$A$-AFM and FM). To evaluate the on-site SIA interaction $K$, only one $Fe^{3+}$ cation was kept while the surrounding $Fe^{3+}$ atoms were replaced by neutral and isoelectronic $Al^{3+}$ cations, which is the same technique that was successfully used for $BiFeO_3$ [4] and $CaMn_7O_{12}$ [6]. The DM parameter $\boldsymbol{D}$ was estimated by replacing all except for four of $Fe^{3+}$ cations with $Al^{3+}$ [4] in an 80 atom unit cell.

As shown in Tab. I, the LSDA+$U$ results show excellent agreement with recent neutron-scattering measurements [7] except for an overestimation of $J_1$.

TABLE I: **Magnetic interaction parameters (meV) compared to neutron-scattering measurements [7, 8].** $D_{\rm AFD}$ splits into two components parallel ($A$=0.042) and perpendicular ($B$=0.075) to spin bond direction.

| meV | $J_1$ | $D=\sqrt{3/2}D_{\rm FE}$ | $D_{\rm AFD}$ | $K$ |
|---|---|---|---|---|
| LSDA+$U$ | -6.1 | 0.109 | 0.075, 0.042 | $3.5\times 10^{-3}$ |
| Neutron | -5.3 | 0.126 | 0.064 | $4.1\times 10^{-3}$ |

## II. Exchange-Striction Polarization driven by AFD.

The AFD rotation ($R_4^+[111]$) breaks the local inversion symmetry between two nearest-neighbor spins. For an AFD rotation, each oxygen moves along [0,$\bar{1}$,1], [1,0,$\bar{1}$], and [$\bar{1}$,1,0], perpendicular to $\mathbf{z}'$ as shown in Fig. 1. Parallel to the oxygen displacements, the local polarization induced by ES is then

$$C_{\rm AFD}\,\mathbf{S}_i\,\mathbf{S}_{i+x}=P_z-P_y \qquad (\text{by O}_x), \tag{17}$$
$$C_{\rm AFD}\,\mathbf{S}_i\,\mathbf{S}_{i+y}=P_x-P_z \qquad (\text{by O}_y), \tag{18}$$
$$C_{\rm AFD}\,\mathbf{S}_i\,\mathbf{S}_{i+z}=P_y-P_x \qquad (\text{by O}_z). \tag{19}$$

Since AFD rotations change sign between layers, the ESP driven by AFD rotations is

$$\boldsymbol{P}^{\rm ES}_{\rm AFD}=C_{\rm AFD}\,\mathbf{z}'\times\mathbf{W}_2, \qquad W_{2k}=\frac{1}{N}\sum_{\mathbf{R}_i,\mathbf{R}_j=\mathbf{R}_i+\mathbf{e}_k}(-1)^{n_i}\,\mathbf{S}_i\cdot\mathbf{S}_j, \tag{20}$$

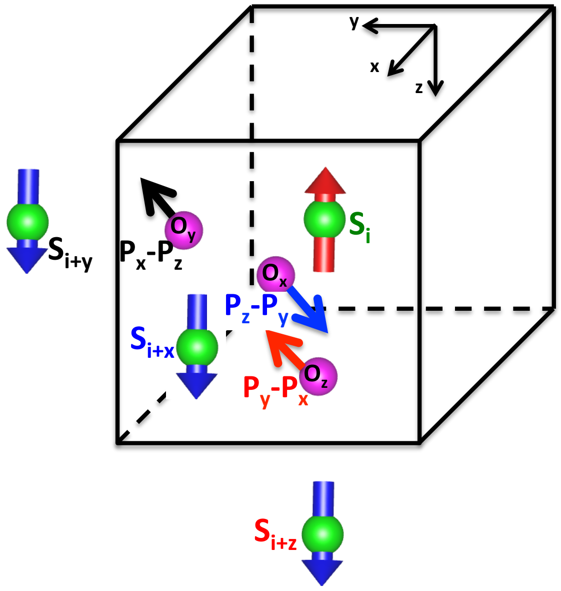


FIG. 1: **Direction of ESP driven by AFD rotation.** Cyan and green atoms represent O and Fe atoms, respectively. Arrows on the O represent the AFD rotation direction.

### III. Spin-Current Polarization Components in Cartesian Axis for $R3c$ $\mathbf{BiFeO_3}$

Defining $\mathbf{f}^{k\gamma} = \frac{\partial \boldsymbol{D}_{\mathrm{FE},k}}{\partial E_\gamma}$ (f denotes FE),

$$\boldsymbol{D}_{\mathrm{FE},x} = (0, D, -D), \qquad \boldsymbol{D}_{\mathrm{FE},y} = (-D, 0, D), \qquad \boldsymbol{D}_{\mathrm{FE},z} = (D, -D, 0) \tag{21}$$

$$\mathbf{f}^{xx} = (0, f, -f), \qquad \mathbf{f}^{yx} = (-g, 0, -h), \qquad \mathbf{f}^{zx} = (g, h, 0), \tag{22}$$

$$\mathbf{f}^{xy} = (0, g, h), \qquad \mathbf{f}^{yy} = (-f, 0, f), \qquad \mathbf{f}^{zy} = (-h, -g, 0), \tag{23}$$

$$\mathbf{f}^{xz} = (0, -h, -g), \qquad \mathbf{f}^{yz} = (h, 0, g), \qquad \mathbf{f}^{zz} = (f, -f, 0), \tag{24}$$

where $f \equiv f^{xx}_y, g \equiv f^{xy}_y$, and $h \equiv f^{xy}_z$.

Defining $\mathbf{a}^{k\gamma} = \frac{\partial \boldsymbol{D}_{\mathrm{AFD},k}}{\partial E_\gamma}$ (a denotes AFD),

$$\boldsymbol{D}_{\mathrm{AFD},x} = (A, B, B), \qquad \boldsymbol{D}_{\mathrm{AFD},y} = (B, A, B), \qquad \boldsymbol{D}_{\mathrm{AFD},z} = (B, B, A), \tag{25}$$

$$\mathbf{a}^{xx} = (a, b, b), \qquad \mathbf{a}^{yx} = (d, c, e), \qquad \mathbf{a}^{zx} = (d, e, c), \tag{26}$$

$$\mathbf{a}^{xy} = (c, d, e), \qquad \mathbf{a}^{yy} = (b, a, b), \qquad \mathbf{a}^{zy} = (e, d, c), \tag{27}$$

$$\mathbf{a}^{xz} = (c, e, d), \qquad \mathbf{a}^{yz} = (e, c, d), \qquad \mathbf{a}^{zz} = (b, b, a), \tag{28}$$

where $a \equiv a^{xx}_x, b \equiv a^{xx}_y, c \equiv a^{xy}_x, d \equiv a^{xy}_y$, and $e \equiv a^{xy}_z$.

Using all the ME couplings derived from the DM interactions altered by an $E$-field,

$$P^{\mathrm{SC}}_x = \sum_x (\mathbf{f}^x_x + \mathbf{a}^x_x)\mathbf{Q}_x + \sum_y (\mathbf{f}^y_x + \mathbf{a}^y_x)\mathbf{Q}_y + \sum_z (\mathbf{f}^z_x + \mathbf{a}^z_x)\mathbf{Q}_z, \tag{29}$$

$$P^{\mathrm{SC}}_y = \sum_x (\mathbf{f}^x_y + \mathbf{a}^x_y)\mathbf{Q}_x + \sum_y (\mathbf{f}^y_y + \mathbf{a}^y_y)\mathbf{Q}_y + \sum_z (\mathbf{f}^z_y + \mathbf{a}^z_y)\mathbf{Q}_z, \tag{30}$$

$$P^{\mathrm{SC}}_z = \sum_x (\mathbf{f}^x_z + \mathbf{a}^x_z)\mathbf{Q}_x + \sum_y (\mathbf{f}^y_z + \mathbf{a}^y_z)\mathbf{Q}_y + \sum_z (\mathbf{f}^z_z + \mathbf{a}^z_z)\mathbf{Q}_z, \tag{31}$$

where $\mathbf{Q}_\gamma = \mathbf{S_i} \times \mathbf{S_{i+\gamma}}$.

## IV. Spin-driven Polarizations from Elastic Neutron Scattering

In order to calculate the spin-driven polarizations from elastic neutron scattering around $T_{\rm N}$, we assume that each of the $\mathbf{z}'$(Fe), $\mathbf{z}'$(Bi) positions along [111] with rotation angle ($\theta$) perpendicular to [111] follows the temperature dependence of the ferroelectric (FE) transition in their Ginzburg-Landau (GL) free energies ($E_{\rm Fe}$, $E_{\rm Bi}$, $E_\theta$) with $T_c$ = 1100 K.

$$E(x) = A(T_c - T)x^2 + Bx^4 + C, \quad x = \mathbf{z}'_{\rm Fe}, \mathbf{z}'_{\rm Bi}, \theta. \tag{32}$$

Since the GL does not include the ME coupling terms, the spin-driven (mostly ES) polarizations along $\mathbf{z}'$ are given by

$$P_{\rm Fe} = Z^*_{\rm Fe}(\mathbf{z}'_{\rm Fe}(\exp) - \mathbf{z}'_{\rm Fe}({\rm GL}))/V, \tag{33}$$
$$P_{\rm Bi} = Z^*_{\rm Bi}(\mathbf{z}'_{\rm Bi}(\exp) - \mathbf{z}'_{\rm Bi}({\rm GL}))/V, \tag{34}$$
$$P_{\rm tot} = P_{\rm Fe} + P_{\rm Bi}. \tag{35}$$

where $V$ is the volume. The effective charges ($Z^*_{\rm Fe/Bi}$=3.81e/4.91e) are calculated using Berry phase polarization theory [9]. $\mathbf{z}'_{Fe/Bi}$ (exp) is the atomic Fe/Bi position along [111] with respect to the oxygen hexagonal plane, and $\mathbf{z}'$(GL) is the free-energy result from Eq. 32 which does not include the ME coupling terms. Therefore the difference $\mathbf{z}'_{\rm Fe/Bi}$(GL)-$\mathbf{z}'_{\rm Fe/Bi}$(exp) represents the spin-driven Bi/Fe displacement with respect to the oxygen plane.

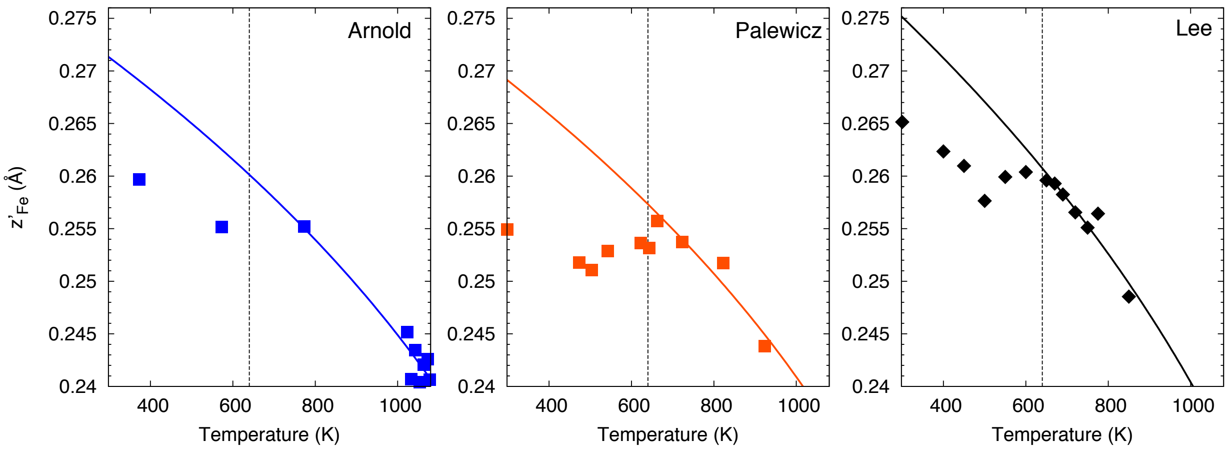


FIG. 2: **ES polarizations due to Fe shifts from neutron scattering measurements.** Elastic neutron-scattering data for Fe-shift from Arnold *et al.*, Palewicz *et al.*, and Lee *et al* as cited in the paper. They are compared with results from GL free energies with the ferroelectric transition temperature $T_{\rm C}$=1100 K. The difference between free energy and neutron-scattering results shows the effect of the spin-driven distortions.

[1] R.S. Fishman, J.T. Haraldsen, N. Furukawa, N. and S. Miyahara, *Phys. Rev. B* **87**, 134416 (2013).
[2] R.S. Fishman, *Phys. Rev. B* **87**, 224419 (2013).
[3] C. Ederer and N.A. Spaldin, Phys. Rev. B **71**, 060401(R) (2005).
[4] C. Weingart, N. Spaldin, and E. Bousquet, Phys. Rev. B **86**, 094413 (2012).

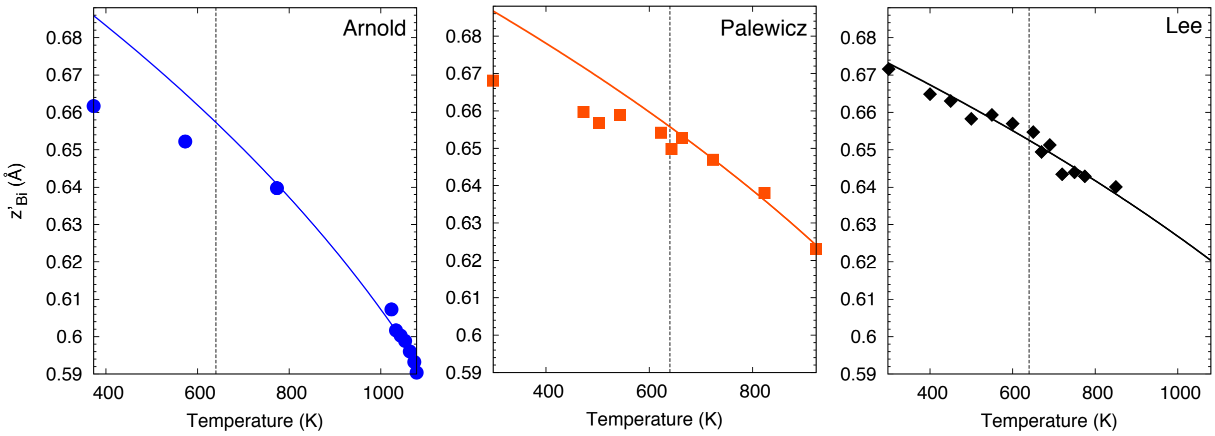


FIG. 3: **ES polarizations due to Bi shifts from neutron-scattering measurements.** Elastic neutron-scattering data for Bi-shift from Arnold *et al.*, Palewicz *et al.*, and Lee *et al* as cited in the paper, again compared with results from the GL free energies. The difference between free energy and neutron-scattering results shows the effect of the spin-driven distortions.

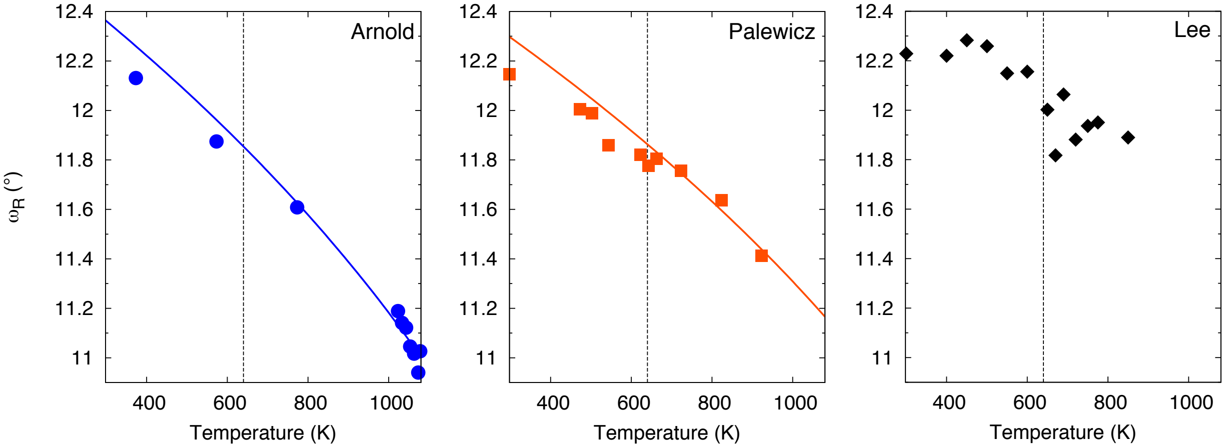


FIG. 4: **ES polarizations due to the change in the AFD rotation ($R_4^+[111]$) from neutron-scattering measurements.** Elastic neutron-scattering data for the change in AFD rotation angles from Arnold *et al.*, Palewicz *et al.*, and Lee *et al* as cited in the paper, again compared with results from the GL free energies. The difference between free energy and neutron-scattering resuls shows the effect of the spin-driven distortions. Free energy data fitting to Lee *et al.* was not shown because of the large scattering in the measurements.


[5] P.E. Blöchl, Phys. Rev. B **50**, 17953 (1994); G. Kresse and D. Joubert, Phys. Rev. B **59**, 1758 (1999).

[6] J.T. Zhang *et al.*, Phys. Rev. B **87**, 075127 (2013).

[7] Nagel, U. *et al.* Terahertz Spectroscopy of Spin Waves in Multiferroic $BiFeO_3$ in High Magnetic Fields. *Phys. Rev. Lett.* **110**, 257201 (2013).

[8] In previous work (M. Matsuda *et al.*, Phys. Rev. Lett. **109**, 067205 (2012)), the spin-wave frequencies were scaled by $\sqrt{S(S+1)}$. This artificial introduction of quantum fluctuations made it awkward to obtain the correct spin-wave frequencies of the canted AF phase, where the upper mode frequency is proportional to $2\mu_B H$ rather than $2\mu_B\sqrt{(S+1)/S}H$. In the present work, the frequencies are scaled by $S$. Consequently, the Heisenberg interactions increase from $J_1 = -4.50$ meV to $J_1 = -5.32$ meV.

[9] R.D. King-Smith and D. Vanderbilt, Theory of polarization of crystalline solids. *Phys. Rev. B* **47**, 1651 (1993).
